# Supplementary material for: EgoGen: An Egocentric Synthetic Data Generator
Source: arXiv:2401.08739 source file (2026-11-04)
Supplement: Supplementary file 1 [file appendix.tex]

\PassOptionsToPackage{table}{xcolor}
\documentclass[10pt,twocolumn,letterpaper]{article}
\usepackage{cvpr}              %
\input{preamble}

\definecolor{cvprblue}{rgb}{0.21,0.49,0.74}
\usepackage[accsupp]{axessibility}
\usepackage[pagebackref,breaklinks,colorlinks,citecolor=cvprblue,hypertexnames=false]{hyperref}

\def\paperID{7475} %
\def\confName{CVPR}
\def\confYear{2024}

\title{EgoGen: An Egocentric Synthetic Data Generator}



\begin{document}



\input{sec/s1_related_work}
\input{sec/s2_egomotion}
\input{sec/s3_egogen}
\input{sec/s4_eval}
\input{sec/s5_lamar}
\input{sec/s6_egoego}
\input{sec/s7_hmr}

\clearpage
{
    \small
    \bibliographystyle{ieeenat_fullname}
    \bibliography{main}
}


\end{document}
